# Supplementary material for: Towards vision-based robotic skins: a data-driven, multi-camera tactile sensor
Source: arXiv:1910.14526 ancillary file (2020-06-23)
Supplement: Supplementary file 1 [file OnlineAppendix.pdf]

# Towards vision-based robotic skins: a data-driven, multi-camera tactile sensor

## Online appendix

Camill Trueeb, Carmelo Sferrazza and Raffaello D’Andrea

### On the thickness of vision-based tactile sensors

In the following, an ideal pinhole camera model and a one-dimensional particle layer are assumed. The size of an image sensor is considered fixed, while the distance of the pinhole with respect to both the image sensor and the particle layer is a design variable.

Let  $f$  denote the focal length, that is, the distance from the image plane to the pinhole, and  $d_0$  the distance from the pinhole to the particle layer, see Figure 1. In order to cover a contiguous planar surface, the field of view (FOV) of the camera is required to be larger than the image sensor’s size, so that multiple cameras may be placed adjacently. This is only valid for  $d_0 \geq f$ .

For  $d_0 \geq f$ , the projection of the observed object on the image sensor will have a size smaller or equal than the object itself. For the sake of simplicity, assume that two particles are distinguishable if they fully lie in two distinct pixels. Therefore, for each particle to be distinguishable in the image, the diameter of a particle,  $d_p$ , needs to have at least the same size as the image sensor’s pixel size,  $\bar{p}$ . The pixel size is generally given in the camera datasheet and it is in the order of few micrometers in modern image sensors. Under the previous constraint, the spatial resolution of the tactile sensor (related to the number of particles) is maximized by setting  $d_p = \bar{p}$ .

As shown in Figure 1, for  $d_0 > f$ , a particle is projected on the image sensor with a reduction in size. In that case, for  $d_p = \bar{p}$ , it covers less than a pixel and may result in being not distinguishable from the others. Therefore, in the rest of the derivation assume,

$$d_0 = f. \tag{1}$$

Theoretically, the distance between the image sensor and the particle layer, that is  $d_0 + f$ , may be arbitrarily small, as long as (1) is satisfied.

Consider now the space needed for a particle to move in the vertical direction, towards the pinhole. Assume that each particle fully lies inside a pixel. Excluding the degenerate case of a particle placed on the optical axis, consider the worst case of a particle placed at the pixel next to the one intersected by the optical axis. From the drawing in Figure 2,

$$\frac{\bar{p} + \Delta x}{d_0} = \frac{\Delta x}{\Delta z} \tag{2}$$

where  $\Delta z$  is the vertical movement of the particle and  $\Delta x$  is the corresponding horizontal displacement (the same in both the image sensor and the particle layer), that is,

$$\Delta x = \frac{\bar{p}\Delta z}{d_0 - \Delta z}. \quad (3)$$

$\Delta x$  is distinguishable in the image if it is at least the size of a pixel, that is,

$$\Delta x \geq \bar{p}, \quad (4)$$

which leads to

$$\Delta z \geq \frac{d_0}{2}. \quad (5)$$

Note that it also holds that  $\Delta z < d_0$ , because of the geometric constraints and to ensure that (3) is valid. Since  $d_0$  can be arbitrarily small, the same applies to  $\Delta z$ .

This analysis shows that in this simplified pinhole scenario, excluding practical and manufacture considerations, the optics does not contribute to a theoretical lower bound on the thickness of a vision-based tactile sensor. Considering that the soft material thickness may also be drastically reduced depending on the application, the main contribution to the thickness is given by the size of image sensor. In this regard, image sensors with a thickness of about 0.3 mm are available on the market. The smallest commercial camera module<sup>1</sup> has a thickness of 1.158 mm, inclusive of a lens, with the possibility of focusing a surface placed at a distance of 3 mm. Such a design may already result in a tactile sensor thickness of about 5 mm.

---

<sup>1</sup><https://www.ovt.com/sensors/OVM6948>

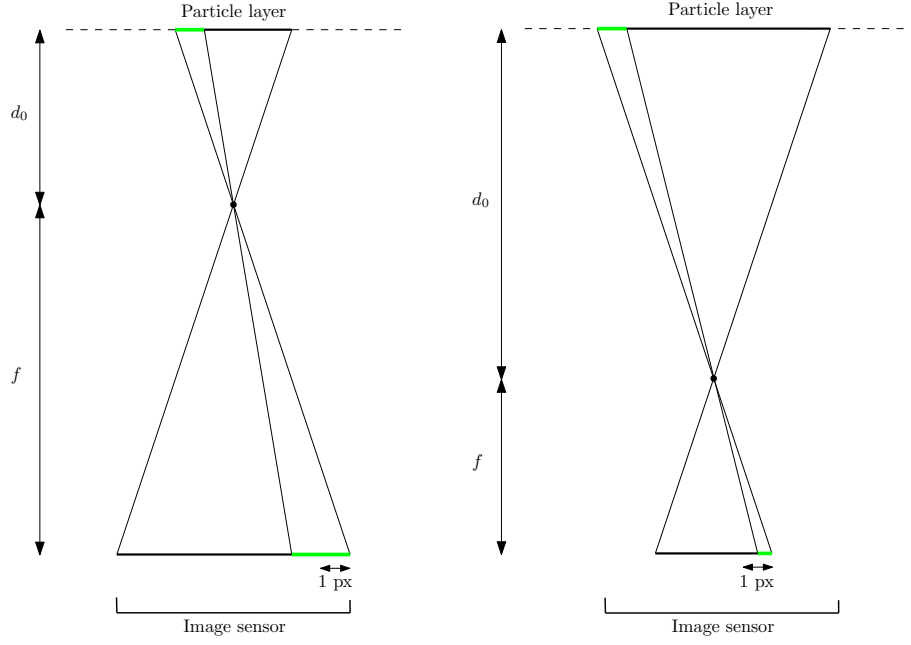

Figure 1: A scheme is shown in this figure with two examples of the resulting FOV and the projection of a particle originally of size  $\bar{p}$  (in green) on the image sensor, for varying  $d_0$  and  $f$ .

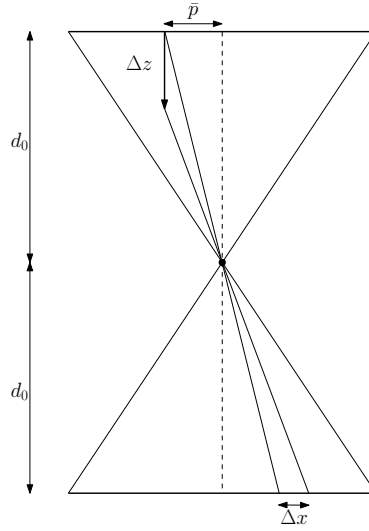

Figure 2: This figure shows a scheme of the projection according to the pinhole camera model, when a particle placed at a distance  $\bar{p}$  from the optical axis (dashed) moves vertically towards the pinhole.
